# Supplementary material for: Ultrafast electron dynamics in platinum and gold thin films driven by optical and terahertz fields
Source: arXiv:2106.10009 ancillary file (2021-08-19)
Supplement: Supplementary file 1 [file SupplementaryMaterial.pdf]

# Supplementary Material
# Ultrafast electron dynamics in platinum and gold thin films driven by optical and terahertz fields

V. Unikandanunni,[1] M.C. Hoffmann,[2] P. Vavassori,[3] S. Urazhdin,[4] and S. Bonetti[1, 5, a)]
[1)]*Department of Physics, Stockholm University, SE-10691 Stockholm, Sweden*
[2)]*Linear Coherent Light Source, SLAC National Accelerator Laboratory, 94025 Menlo Park, CA, USA*
[3)]*CIC nanoGUNE BRTA, San Sebastian, and IKERBASQUE, Basque Foundation for Science, Bilbao, Spain*
[4)]*Department of Physics, Emory University, Atlanta, GA, USA*
[5)]*Department of Molecular Sciences and Nanosystems, Ca' Foscari University of Venice, 30172 Venice, Italy*

## I. TWO-TEMPERATURE MODEL SIMULATIONS

We used the open-source python-based simulation package NTMpy to both solve the two-temperature model (2TM) for our material, as well as to calculate the absorbed fluence using the transfer matrix method[1]. The optical excitation was modelled with as a Gaussian-like pulse with the experimental measured with, whereas the terahertz excitation was mimicking the experimental the shape of the electric field recorded with electro-optical sampling. The physical parameters used for the 2TM simulations are reported in Table I. All the parameters are taken from the literature except for the THz refractive index which was not available, hence we measured it using the THz time-domain spectroscopy method, as described in the next section. The electron-phonon coupling $G$ was found overlapping the 2TM simulations with the experimental data. This is justified assuming a linear relationship between the reflectivity change and the weighted sum of the electronic and the lattice temperature change following the procedure given in Ref.[2].

TABLE I. Table containing values of parameters used for Two-temperature model simulations

| | Platinum[3–7] | Gold[3,8–13] | Silicon[14–17] |
|---|---|---|---|
| $C_e$(J/m$^3$K) | $740\times T_e$ | $71\times T_e$ | $50\times T_e$ |
| $C_l$(J/m$^3$K) | $2.78\times10^6$ | $2.49\times10^6$ | $2.237\times10^6$ |
| $k_e$(W/mK) | 18 | 315 | $25\times10^{-6}T_e$ |
| $k_l$(W/mK) | 6.7 | 2.6 | 130 |
| G(W/m$^3$K)[a] | $(2.5–11)\times10^{17}$ | $(2.1\pm0.3)\times10^{17}$ | $2.8\times10^{17}$ |
| $\rho$(kg/m$^3$) | $21.4\times10^3$ | $19.3\times10^3$ | $2.33\times10^3$ |
| $n_{800}$ | $2.85+4.96j$ | $0.15+4.91j$ | $3.69+0.0066j$ |
| $n_{THz}$[b] | $70+135j$ | $5.3+70j$ | 3.42 |

[a] The literature value was taken as the initial guess before fine-tuning

## II. THZ TIME-DOMAIN SPECTROSCOPY SAMPLE CHARACTERIZATION

Fig.1(a) shows the terahertz transmission through the different samples. The relatively high THz transmission in gold indicates that the film thickness is at the percolation threshold[18,19]. The complex refractive index in Fig.1(b) is extracted from the measured terahertz transmission using the Tinkham formula[20,21]

$$\widetilde{n}^2(\omega) = 1 + i\frac{(1+n_s)c}{d\omega}\left(\frac{1}{\widetilde{T}(\omega)} - 1\right), \tag{1}$$

[a)]Electronic mail: stefano.bonetti@fysik.su.se

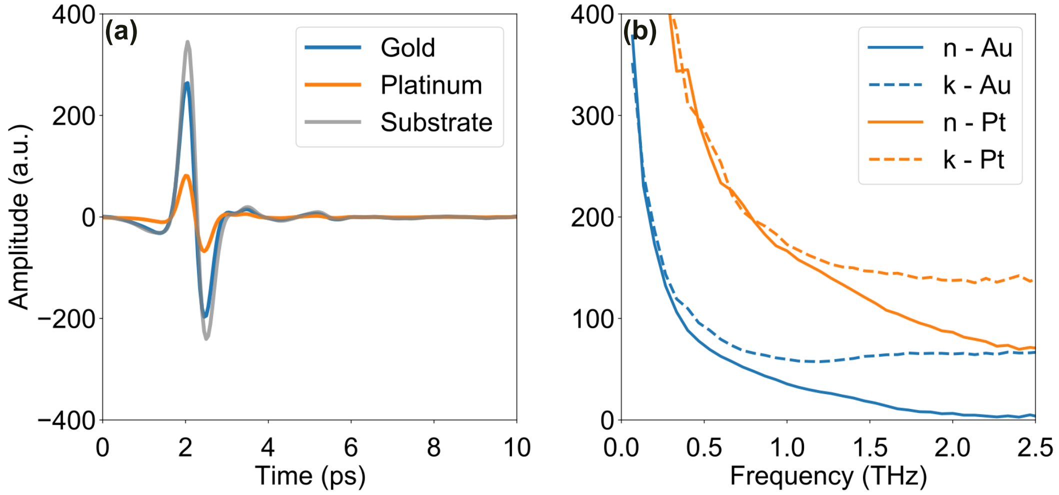


FIG. 1. (a) Terahertz time-domain transmission traces of gold and platinum thin films, and for the silicon substrate. (b) Extracted real and imaginary part of the refractive index platinum and gold.

where $\widetilde{n}(\omega)$ is the complex refractive index of the film, $\widetilde{T}(\omega)$ is the complex transmittivity in frequency domain, $n_s$ is the refractive index of the substrate, $d$ is the thickness of the sample, and $c$ is the speed of light. $\widetilde{T}(\omega)$ is computed as the Fourier transform of the electric field transmitted by the sample on the substrate, divided it by the Fourier transform of the electric field transmitted by the bare substrate. Below $\sim 0.5$ THz the phase is typically not reliably measured with this technique, hence we in that region we used data linearly extrapolated from the higher frequency values, following a standard procedure[22].

## III. TRANSIENT OPTICAL REFLECTIVITY AND MATERIAL PROPERTIES

The reflectivity $R$ for a beam impinging normally on a semi-infinite medium with refractive index $\tilde{n} = n + ik$ is

$$R = \frac{(n-1)^2 + k^2}{(n+1)^2 + k^2}. \tag{2}$$

The relative change of reflectivity $\Delta R/R$ can be written as a function of the change in the real and imaginary parts of the dielectric constant $\tilde{\varepsilon} = \varepsilon_1 + i\varepsilon_2$, i.e.

$$\frac{\Delta R}{R} = \frac{1}{R}\left(\frac{\partial R}{\partial n}\frac{\partial n}{\partial \varepsilon_1} + \frac{\partial R}{\partial k}\frac{\partial k}{\partial \varepsilon_1}\right)\Delta\varepsilon_1 + \frac{1}{R}\left(\frac{\partial R}{\partial n}\frac{\partial n}{\partial \varepsilon_2} + \frac{\partial R}{\partial k}\frac{\partial k}{\partial \varepsilon_2}\right)\Delta\varepsilon_2 \tag{3}$$

By evaluating the terms in the brackets, Eq. (3) can be expanded as

$$\frac{\Delta R}{R} = \left\{\frac{n}{n^2+k^2}\left(\frac{n-1}{(n-1)^2+k^2} - \frac{n+1}{(n+1)^2+k^2}\right) - \frac{k}{n^2+k^2}\left(\frac{k}{(n-1)^2+k^2} - \frac{k}{(n+1)^2+k^2}\right)\right\}\Delta\varepsilon_1 + \left\{\frac{k}{n^2+k^2}\left(\frac{n-1}{(n-1)^2+k^2} - \frac{n+1}{(n+1)^2+k^2}\right) + \frac{n}{n^2+k^2}\left(\frac{k}{(n-1)^2+k^2} - \frac{k}{(n+1)^2+k^2}\right)\right\}\Delta\varepsilon_2 \tag{4}$$

The coefficients of $\Delta\varepsilon_1$ and $\Delta\varepsilon_2$ are often denoted as $\alpha$ and $\beta$ respectively and are known as Seraphin's coefficients[23]. For our gold films $\alpha \approx -0.0014$ and $\beta = -0.016$, i.e. both of them are negative with $|\alpha| < |\beta|$. This is important for the considerations later on.

In order to understand what causes the transient optical reflectivity, we need to express the variation of the complex dielectric function, i.e. $\Delta\varepsilon_1$ and $\Delta\varepsilon_2$ in terms of characteristic material parameters. We chose Drude-Lorentz model[24] with two Lorentz

oscillators as a good approximation for the dielectric function of our gold films. The dielectric function $\tilde{\varepsilon}(\omega)$ is then

$$\tilde{\varepsilon}(\omega) = 1 - \frac{\omega_p^2}{\omega^2 + i\omega\gamma} + \omega_p^2 \sum_{j=1}^{2} \frac{f_j}{\omega_j^2 - \omega^2 - i\omega\gamma_j}, \tag{5}$$

where $\omega_p$ is the plasma frequency, $\omega_j$ is the resonance frequency, $f_j$ is the oscillator strength, $\gamma_j$ is the electron-electron scattering rate. The first term in Eq. (5) is the free electron contribution to the dielectric function, whereas the second term denotes the contribution from two interband transitions. The dielectric response at near-infrared frequencies is dominated by the free electron absorption[25]. However, interband transitions close by the probing energy can also have a measurable effect.

The the two interband transitions are both transitions from the $d-$band to the Fermi-surface. The first one is a weak transition near the $X$ symmetry point and at approximately 1.9 eV, while the second is the dominant transition close to the $L$ point, and it has a resonance energy of 2.4 eV. These two transitions are both close to our probe energy of 1.55 eV, hence they can affect the reflectivity[26]. The real and imaginary parts of the dielectric function given in Eq. (5) are then

$$\varepsilon_1(\omega) = 1 - \frac{\omega_p^2}{\omega^2 + \gamma^2} + \omega_p^2 \sum_{j=1}^{2} \frac{f_j(\omega_j^2 - \omega^2)}{(\omega_j^2 - \omega^2)^2 + \omega^2\gamma_j^2} \tag{6}$$

$$\varepsilon_2(\omega) = \frac{\omega_p^2\gamma}{\omega(\omega^2 + \gamma^2)} + \omega_p^2\omega \sum_{j=1}^{2} \frac{f_j\gamma_j}{(\omega_j^2 - \omega^2)^2 + \omega^2\gamma_j^2} \tag{7}$$

The variation of the real and imaginary parts of $\varepsilon$ at a given frequency $\omega$ can hence be due either to a change in $\omega_p$ or in $\gamma$, induced by the pump field[27]. This is based on the assumption that the pump has a negligible effect on the oscillator strength, on the resonance frequency and on the scattering rates of bound electrons. This is a reasonable assumption since in a metal they are well screened by the free electrons. Hence we can write

$$\Delta\varepsilon_1 = A_1\Delta\omega_p + B_1\Delta\gamma \tag{8}$$

$$\Delta\varepsilon_2 = A_2\Delta\omega_p + B_2\Delta\gamma \tag{9}$$

Differentiating Eqs. (6) and (7) with respect to $\omega_p$ and $\gamma$ gives the explicit expressions for $A_1$,$B_1$,$A_2$, and $B_2$, i.e.

$$A_1 = \frac{-2\omega_p}{\omega^2 + \gamma^2} + 2\omega_p \sum_{j=1}^{2} \frac{f_j(\omega_j^2 - \omega^2)}{(\omega_j^2 - \omega^2)^2 + \omega^2\gamma_j^2}, \quad B_1 = \frac{2\omega_p^2\gamma}{(\omega^2 + \gamma^2)^2} \tag{10}$$

$$A_2 = \frac{2\omega_p\gamma}{\omega(\omega^2 + \gamma^2)} + 2\omega_p\omega \sum_{j=1}^{2} \frac{f_j\gamma_j}{(\omega_j^2 - \omega^2)^2 + \omega^2\gamma_j^2}, \quad B_2 = \frac{\omega_p^2(\omega^2 - \gamma^2)}{\omega(\omega^2 + \gamma^2)^2} \tag{11}$$

### A. 800 nm driven dynamics

Given that $\omega_p = \sqrt{Ne^2/\varepsilon_0 m}$, where $N$ is the free electron density, $e$ is the electronic charge, $\varepsilon_0$ is the vacuum permittivity and $m$ is the mass of electron, a variation in the plasma frequency can be ascribed only with a variation in $N$. With the optical pump fields used in the experiments presented in the main text, i.e. at 1.55 eV, below the photoemission threshold, $N$ is expected to stay constant. Hence, the change in $\tilde{\varepsilon}$ in this case must be ascribed to a variation of the scattering rate. Such variation is in turn related to the change in electronic and lattice temperatures $T_e$ and $T_l$ according to the expression[25]

$$\Delta\gamma = 2A_{ee}T_e\Delta T_e + B_{ep}\Delta T_l, \tag{12}$$

where $A_{ee} = 1.7 \times 10^7 s^{-1}K^{-2}$ and $B_{ep} = 1.45 \times 10^{11} s^{-1}K^{-2}$ are the electron-electron and, respectively, the electron-phonon scattering coefficients for gold, implying $\Delta\gamma > 0$. From Eqs. (10) and (11), we see that $B_1, B_2 > 0$ if $\omega^2 > \gamma^2$. This is true in our case, since $\hbar\omega = 1.55$ eV and $\hbar\gamma \approx 0.1$ eV.

Thus, the variation of both the real and imaginary parts of the dielectric constant is positive, i.e. $\Delta\varepsilon_1, \Delta\varepsilon_2 > 0$. This situation, combined with the negative values of the Seraphin's coefficients $\alpha$ and $\beta$ discussed above, leads to a negative transient reflectivity change, i.e. $\Delta R/R < 0$ for 800 nm pump-probe experiments. This is consistent with the observation in the main text. An advanced quantum mechanical treatment of the thermal modulation of the dielectric constant can be found in the work of Conforti et al[26].

### B. THz driven dynamics

In the main text, we argued that the THz pump induced field emission of electrons via Fowler-Nordheim tunneling. If electrons are emitted, the free electron concentration $N$ is reduced, which in turn would reduce the plasma frequency $\omega_p$ as discussed in the previous section. More precisely

$$\frac{\Delta\omega_p}{\omega_p} = \frac{\Delta N}{2N} \tag{13}$$

$A_2$ in Eq. (11) is always positive since all terms in the expressions are positive. On the contrary, $A_1$ can have positive or negative depending on the relative weight of the free electron term to the interband one. Assuming $f_j = 1$, $A_1 > 0$, but even with a smaller oscillator strength, a positive $A_1$ is expected when including contributions from all the interband transitions[28]. With $A_1, A_2 > 0$ and $\Delta\omega_p < 0$, $\Delta\varepsilon_1 > 0$ which, combined with the first Seraphine's coefficient $\alpha < 0$, result in a positive reflectivity change $\Delta R/R > 0$, as we report in the main text.

We have neglected in this last consideration the role of the electron-electron scattering rate. In the initial part of the THz-induced dynamics, $\Delta\gamma \approx 0$, since the THz energy is dissipated as kinetic energy of the emitted electrons rather than in thermalization, which occurs at later time scales. In the main text, we indeed report a small negative reflectivity change $\Delta R/R < 0$ in the later part of dynamics, which is consistent with $\Delta\gamma > 0$ and the same reasoning as for the 800 nm pump data.

## IV. THZ TRANSIENT REFLECTIVITY IN 50 NM FILMS

As complementary measurements, we show here the transient reflectivity driven by the THz pump on thicker (50 nm) platinum and gold films, and we compare them with the main text data in Fig. 2(a)-(b) taken on 10 nm thick films. The thicker platinum film shows a 25 times smaller reflectivity variation, and no observable signal can be measured from the thicker gold film. In Fig. 3, we compare the absorption profiles of the two materials and for the two thicknesses, using the transfer matrix method. For both materials, we observe a much lower absorption for the thicker films.

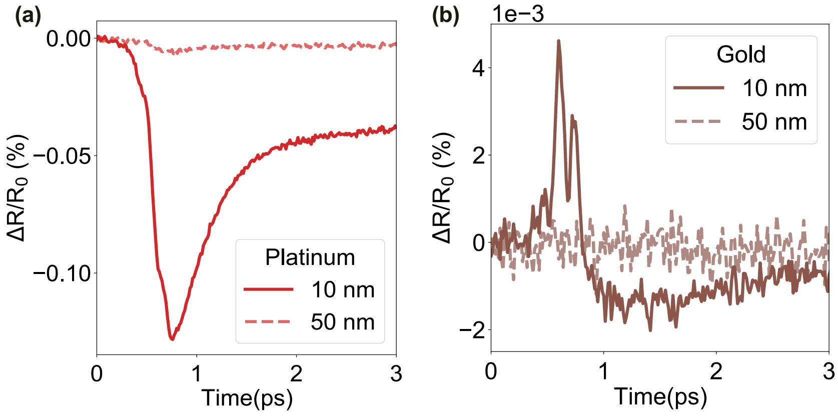


FIG. 2. Comparison of the THz-induced transient reflectivity in (a) platinum and (b) gold thin films of different thickness, all grown on a silicon substrate.

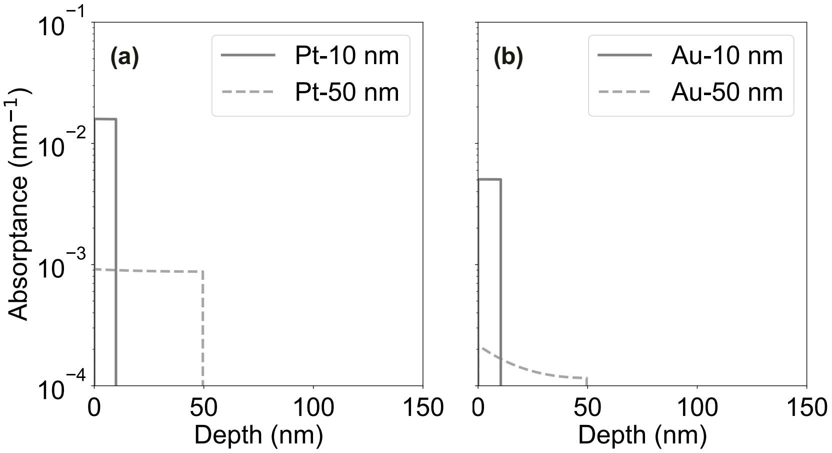


FIG. 3. THz absorption profile calculated using the transfer matrix method for (a) platinum and (b) gold films of different thickness

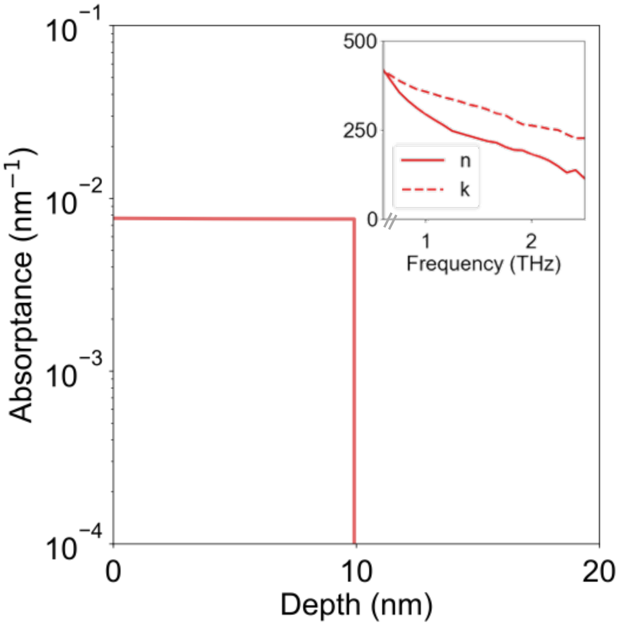


FIG. 4. THz absorption profile calculated using the transfer matrix method for sputtered gold film of thickness 10 nm. Inset: real (n) and imaginary (k) part of refractive index as a function of frequency measured using time-domain THz spectroscopy

[1]"NTMpy-N-Temperature Model solver," `https://github.com/udcm-su/NTMpy`.

[2]S. Brorson, A. Kazeroonian, J. Moodera, D. Face, T. Cheng, E. Ippen, M. Dresselhaus, and G. Dresselhaus, "Femtosecond room-temperature measurement of the electron-phonon coupling constant $\gamma$ in metallic superconductors," Physical Review Letters **64**, 2172 (1990).

[3]J. Hohlfeld, S.-S. Wellershoff, J. Güdde, U. Conrad, V. Jähnke, and E. Matthias, "Electron and lattice dynamics following optical excitation of metals," Chemical Physics **251**, 237–258 (2000).

[4]A. D. Rakić, A. B. Djurišić, J. M. Elazar, and M. L. Majewski, "Optical properties of metallic films for vertical-cavity optoelectronic devices," Applied optics **37**, 5271–5283 (1998).

[5]D. E. Gray, "American institute of physics handbook," AmJPh **32**, 389–389 (1964).

[6]Y. Wang, Z. Lu, and X. Ruan, "First principles calculation of lattice thermal conductivity of metals considering phonon-phonon and phonon-electron scattering," Journal of applied Physics **119**, 225109 (2016).

[7]M. Duggin, "The thermal conductivities of aluminium and platinum," Journal of Physics D: Applied Physics **3**, L21 (1970).

[8]N. Smirnov, "Copper, gold, and platinum under femtosecond irradiation: Results of first-principles calculations," Physical Review B **101**, 094103 (2020).

[9]D. I. Yakubovsky, Y. V. Stebunov, R. V. Kirtaev, G. A. Ermolaev, M. S. Mironov, S. M. Novikov, A. V. Arsenin, and V. S. Volkov, "Au-mos2 interfaces: Ultrathin and ultrasmooth gold films on monolayer mos2 (adv. mater. interfaces 13/2019)," Advanced Materials Interfaces **6**, 1970082 (2019).

[10]A. Block, M. Liebel, R. Yu, M. Spector, Y. Sivan, F. G. de Abajo, and N. F. van Hulst, "Tracking ultrafast hot-electron diffusion in space and time by ultrafast thermomodulation microscopy," Science advances **5**, eaav8965 (2019).
[11]E. D. Palik, *Handbook of optical constants of solids*, Vol. 3 (Academic press, 1998).
[12]A. P. Caffrey, P. E. Hopkins, J. M. Klopf, and P. M. Norris, "Thin film non-noble transition metal thermophysical properties," Microscale Thermophysical Engineering **9**, 365–377 (2005).
[13]P. B. Johnson and R.-W. Christy, "Optical constants of the noble metals," Physical review B **6**, 4370 (1972).
[14]Z. Kan, Q. Zhu, H. Ren, and M. Shen, "Femtosecond laser-induced thermal transport in silicon with liquid cooling bath," Materials **12**, 2043 (2019).
[15]D. E. Aspnes and A. Studna, "Dielectric functions and optical parameters of si, ge, gap, gaas, gasb, inp, inas, and insb from 1.5 to 6.0 ev," Physical review B **27**, 985 (1983).
[16]J. Dai, J. Zhang, W. Zhang, and D. Grischkowsky, "Terahertz time-domain spectroscopy characterization of the far-infrared absorption and index of refraction of high-resistivity, float-zone silicon," JOSA B **21**, 1379–1386 (2004).
[17]J. Thorstensen and S. Erik Foss, "Temperature dependent ablation threshold in silicon using ultrashort laser pulses," Journal of Applied Physics **112**, 103514 (2012).
[18]K. Yoshioka, Y. Minami, K.-i. Shudo, T. D. Dao, T. Nagao, M. Kitajima, J. Takeda, and I. Katayama, "Terahertz-field-induced nonlinear electron delocalization in au nanostructures," Nano letters **15**, 1036–1040 (2015).
[19]M. Walther, D. Cooke, C. Sherstan, M. Hajar, M. Freeman, and F. Hegmann, "Terahertz conductivity of thin gold films at the metal-insulator percolation transition," Physical Review B **76**, 125408 (2007).
[20]R. Glover III and M. Tinkham, "Conductivity of superconducting films for photon energies between 0.3 and 4 0 k t c," Physical Review **108**, 243 (1957).
[21]A. Paulke, *Transient Conductivity Measurements using Terahertz Time-Domain Spectroscopy*, Ph.D. thesis, PhD thesis, UNIVERSITAT POTSDAM (2013).
[22]L. Duvillaret, F. Garet, and J.-L. Coutaz, "A reliable method for extraction of material parameters in terahertz time-domain spectroscopy," IEEE Journal of selected topics in quantum electronics **2**, 739–746 (1996).
[23]B. Seraphin and N. Bottka, "Band-structure analysis from electro-reflectance studies," Physical Review **145**, 628 (1966).
[24]J. D. Jackson, "Classical electrodynamics," (1999).
[25]A. N. Smith and P. M. Norris, "Influence of intraband transitions on the electron thermoreflectance response of metals," Applied Physics Letters **78**, 1240–1242 (2001).
[26]M. Conforti and G. Della Valle, "Derivation of third-order nonlinear susceptibility of thin metal films as a delayed optical response," Physical Review B **85**, 245423 (2012).
[27]R. Rosei and D. W. Lynch, "Thermomodulation spectra of al, au, and cu," Physical Review B **5**, 3883 (1972).
[28]A. Marini, M. Conforti, G. Della Valle, H. Lee, T. X. Tran, W. Chang, M. Schmidt, S. Longhi, P. S. J. Russell, and F. Biancalana, "Ultrafast nonlinear dynamics of surface plasmon polaritons in gold nanowires due to the intrinsic nonlinearity of metals," New Journal of Physics **15**, 013033 (2013).
